# Supplementary material for: Quantifying Memory Utilization with Effective State-Size
Source: arXiv:2504.19561 source file (2025-04-28)
Supplement: Supplementary file 1 [file _reproducibility.tex]

\section*{Impact Statement}
% this section doesn't count towards page limit

This paper presents work whose goal is to advance the field of Machine Learning. There are many potential societal consequences of our work, none which we feel must be specifically highlighted here.
